# Supplementary material for: Conjunctive Queries with Theta Joins Under Updates
Source: arXiv:1905.09848 source file (2019-05-23)
Supplement: Supplementary file 1 [file gjts_for_cgqs.tex]

%!TEX root = ../main/main.tex

In order to present the construction of a GJT we need to introduce some further notation. Let $A$ be a set of hyperedges and let $\cP$ be a set of predicates. We say that $n\in A$ is connected to $P\in\cP$, denoted by $n\sim P$ if $\var(n)\cap\var(P)\neq\emptyset$. Given two hyperedges $n$ and $m$ in $A$, we say that they are connected by $\cP$, denoted by $n\sim_cP m$ if there is a predicate $P\in\cP$ such that $n\sim P$ and $m\sim P$. We define the vicinity of an hyperedge $n\in A$ under $\cP$ and $A$ as $\vicinity_{\cP}^A(n)=\{m\in A\mid n\sim_{\cP} m\land n\neq m\}$.

We now present an algorithm that, given a GCQ $Q$, returns a bynary GJT for $Q$ if $Q$ is acyclic, and returns \texttt{cyclic} otherwise. Note that by Lemma~\martin{cite lemma} there is no loss of generality. The algorithm works in a recursive manner, maintaining at each step two sets $A$ and $\cP$ of remaining hyperedges and remaining predicates, respectively. $A$ is initialized to $\atoms(Q)$ (considering each atom as a hyperedge with the corresponding set of variables) and $\cP$ to $\predicates(Q)$. At each step of the recursion, the following two invariants are maintained:

\begin{enumerate}
	\item\label{item:prop-connected} $A$ is connected, in the sense that the equivalence relation $\sim_{\cP}$ defines a single partition over $A$.
	\item\label{item:prop-two-atoms} Given a predicate $P\in \cP$, the set $\{n\in A\mid n\sim P\}$ contains exactly two elements.
\end{enumerate}

At the beginning, property~\ref{item:prop-connected} can be assumed true since if a query is acyclic but not connected, we can construct one GJT for each connected component and merge them into a single tree trivially. Property~\ref{item:prop-two-atoms} needs to be checked at the beginning; if a predicate mentions three atoms then the query is cyclic, while predicates mentioning a single atom can be ignored since they do not impose any restriction to GJTs.

The algorithm works as follows: at each recursive step, it chooses nondeterministically a predicate $P\in\cP$ such that either $\vicinity(c_1)=\{c_2\}$ or $\vicinity(c_2)=\{c_1\}$, where $c_1$ and $c_2$ are the only hyperedges in $A$ connected to $P$ (see property~\ref{item:prop-two-atoms}). If such a predicate does not exist, then it returns \texttt{cyclic}. Assume now w.l.o.g that $\vicinity(c_1)=\{c_2\}$, and define $n$ as a new atom containing the set of variables $\var(c_1)\cap\var(\vicinity_{\cP}^A(c_1))$. Add to the resulting tree the node $n$ with $c_1$ and $c_2$ as children; continue recursively with $A=A\setminus\{c_1,c_2\}$ and $\cP=\cP\setminus\{P\}$. The algorithm ends when there is no predicate in $\cP$.
